# Supplementary material for: Bounds on the mosaic number of Legendrian Knots
Source: arXiv:2410.08064 source file (2024-10-10)
Supplement: Supplementary file 1 [file mosaic_catalogs.tex]

{
\raggedcolumns
\setlength{\parskip}{1em}

\begin{multicols}{2}
\resizebox{\linewidth}{!}{
\begin{tabular}{|c|c|r|}
\hline
\multicolumn{3}{|c|}{$0_1$}                          \\
\hline
tb    & rot  & Minimal Mosaic                        \\
\hline
-1    & 0  & 2134                                  \\
-2    & 1  & 021246354                             \\
-3    & 0  & 021284340                             \\
-3    & 2  & 0021024624063554                      \\
-4    & 1  & 0000021028913434                      \\
-4    & 3  & 0002100246024062400635554             \\
-5    & 0  & 0021028428403400                      \\
-5    & 2  & 0210279139840340                      \\
-5    & 4  & 0212128746399162434635554             \\
-6    & 1  & 0021028428913434                      \\
-6    & 3  & 0002100246028162439435540             \\
-6    & 5  & 000000255510621281389846243406355554  \\
-7    & 0  & 2121398428913434                      \\
-7    & 2  & 0000000210027912898434340             \\
-7    & 4  & 000000000021021246279916398846034354  \\
-7    & 6  & 002121028746284606395916240346355554  \\
-8    & 1  & 0000000210028812898434340             \\
-8    & 3  & 0021002791279843984003400             \\
-8    & 5  & 000021000246002816028466243594355540  \\
-9    & 0  & 0000002121288843989103434             \\
-9    & 2  & 0002100284027912898434340             \\
-9    & 4  & 000000000210002871028794243991355434  \\
-9    & 6  & 002121028746287916399846243406355554  \\
-10   & 1  & 0002100284028812898434340             \\
-10   & 3  & 0212127984399712878434340             \\
-10   & 5  & 000021000246002816028794243991355434  \\
-11   & 0  & 0002121284398812898434340             \\
-11   & 2  & 0212127984398712888434340             \\
-11   & 4  & 000000002121027984279971398784034340  \\
-11   & 6  & 002121028746287954379951246624354340  \\
-12   & 1  & 0212127984398812898434340             \\
-12   & 3  & 000000002121027984279871398884034340  \\
-12   & 5  & 000021021246287816379794289791343434  \\
-13   & 0  & 0212128884398812898434340             \\
-13   & 2  & 000000002121027984279881398984034340  \\
-13   & 4  & 000021021246279916398884288891343434  \\
-13   & 6  & 021210287791379984279971398984034340  \\
-14   & 1  & 000000000210212881398884289891343434  \\
-14   & 3  & 000021021246279716398884289891343434  \\
-14   & 5  & 002121027984279971399784287840343400  \\
-15   & 0  & 000000002121028884288881398984034340  \\
-15   & 2  & 000000021210279881398884289891343434  \\
-15   & 4  & 002121027984279871398894288891343434  \\
-16   & 1  & 000000021210288881398884289891343434  \\
-16   & 3  & 000251021624279881398884289891343434  \\
-16   & 5  & 212121398846288816398794243991355434  \\
-17   & 0  & 000021021284287881388884289891343434  \\
-17   & 2  & 000021021284279881398884289891343434  \\
-17   & 4  & 212121397984297881638884629891343434  \\
-18   & 1  & 000021021284288881398884289891343434  \\
-18   & 3  & 002121027984279881398884289891343434  \\
-19   & 0  & 002121028784288881388884289891343434  \\
-19   & 2  & 002121027984288881398884289891343434  \\
-20   & 1  & 002121028884288881398884289891343434  \\
-21   & 0  & 212121398884288881398884289891343434  \\
\hline
\end{tabular}
}

\resizebox{\linewidth}{!}{
\begin{tabular}{|c|c|r|}
\hline
\multicolumn{3}{|c|}{$3_1$}     \\
\hline
tb    & rot  & Minimal Mosaic                        \\
\hline
-6    & 1  & 0021002971294663759403540             \\
-7    & 0  & 0021002971298463791603434             \\
-7    & 2  & 0210028910399710379400340             \\
-8    & 1  & 0021002871298943794003400             \\
-8    & 3  & 000000002100029710243991355984000340  \\
-9    & 0  & 0021002971298843799103434             \\
-9    & 2  & 0021002871298943799103434             \\
-9    & 4  & 000210002460029160243991355984000340  \\
-10   & 1  & 0021025891629843989103434             \\
-10   & 3  & 0021002891289843984003400             \\
-11   & 0  & 000000000210002971029884287991343434  \\
-11   & 2  & 0021002891289843989103434             \\
-11   & 4  & 000000002100028710288991379984034340  \\
-12   & 1  & 2121039891289843989103434             \\
-12   & 3  & 000000000210002891028984289840343400  \\
-12   & 5  & 000210002460028160288991379984034340  \\
-13   & 0  & 000000002121029784298881379984034340  \\
-13   & 2  & 000000000210002891028984289891343434  \\
-13   & 4  & 000000002121028784288991379984034340  \\
-14   & 1  & 000000000210212891398984289891343434  \\
-14   & 3  & 000000002121028984289871398884034340  \\
-14   & 5  & 000210002791028984289971398784034340  \\
-15   & 0  & 000000021210279891398984289891343434  \\
-15   & 2  & 000000002121028984289881398984034340  \\
-15   & 4  & 000021021284287891379984289840343400  \\
-15   & 6  & 021210287791379984289971398784034340  \\
-16   & 1  & 000000021210288891398984289891343434  \\
-16   & 3  & 000021021284287891379984289891343434  \\
-16   & 5  & 002121027984289971399884287840343400  \\
-17   & 0  & 000021021284279891398984289891343434  \\
-17   & 2  & 000021021284287891388984289891343434  \\
-17   & 4  & 002121027984289971399884287891343434  \\
-18   & 1  & 000021021284288891398984289891343434  \\
-18   & 3  & 002100028910289881398884289891343434  \\
-19   & 0  & 002121027984288891398984289891343434  \\
-19   & 2  & 002121028784288891388984289891343434  \\
-20   & 1  & 002121028884288891398984289891343434  \\
-20   & 3  & 002121028984289881398884289891343434  \\
-21   & 2  & 212121398884288891398984289891343434  \\
\hline
\end{tabular}
}

\resizebox{\linewidth}{!}{
\begin{tabular}{|c|c|r|}
\hline
\multicolumn{3}{|c|}{$m(3_1)$}                     \\
\hline
tb    & rot  & Minimal Mosaic                        \\
\hline
1     & 0  & 0021025971629943943103554             \\
0     & 1  & 0021002891299463791603434             \\
-1    & 0  & 0021002891299843794003400             \\
-1    & 2  & 0210028910397912434635554             \\
-2    & 1  & 0021002891299843799103434             \\
-2    & 3  & 000000002100028910284391395546035554  \\
-3    & 0  & 0210028710397912898434340             \\
-3    & 2  & 0212128946397162894634354             \\
-3    & 4  & 000000021210289891397466243546355554  \\
-4    & 1  & 0212128784397912894634354             \\
-4    & 3  & 000000002121028946289716397946034354  \\
-4    & 5  & 002121028946299916639746628406343554  \\
-5    & 0  & 0212128784397912898434340             \\
-5    & 2  & 000000000210212891399984287991343434  \\
-5    & 4  & 000021021246289816397466289546343554  \\
-6    & 1  & 000000002121028784279791398984034340  \\
-6    & 3  & 000000021210289891397974243891355434  \\
-6    & 5  & 002121259746628816639794627991343434  \\
-7    & 0  & 000000002121028784288791398984034340  \\
-7    & 2  & 000000021210287891397974289891343434  \\
-7    & 4  & 000210212791399984279791398984034340  \\
-8    & 1  & 000000021210287881397984289891343434  \\
-8    & 3  & 000021021246289816397794289891343434  \\
-8    & 5  & 021210279791399984279791398984034340  \\
-9    & 0  & 000021021284287791397984289891343434  \\
-9    & 2  & 000021021246289816397884289891343434  \\
-9    & 4  & 002121028946288916397994289891343434  \\
-10   & 1  & 000021021284287881397984289891343434  \\
-10   & 3  & 002121028784287991397974289891343434  \\
-11   & 0  & 002121027984287881397984289891343434  \\
-11   & 2  & 002121028784287981397984289891343434  \\
-12   & 1  & 002121028784288791398884289891343434  \\
-13   & 0  & 212121398784288791398884289891343434  \\
\hline
\end{tabular}%m(3_1)
}

\resizebox{\linewidth}{!}{
\begin{tabular}{|c|c|r|}
\hline
\multicolumn{3}{|c|}{$3_1\#3_1$} \\
\hline
tb    & rot  & Minimal Mosaic                        \\
\hline
-11   & 0  & 255100602910629891398946039406003554  \\
-12   & 1  & 002100258910629891398946039406003554  \\
-13   & 0  & 002100258910629891398946039424003540  \\
-13   & 2  & 002100028910289891398946039406003554  \\
-14   & 1  & 002100028910289891398946039424003540  \\
-15   & 0  & 002100028910289891398984039840003400  \\
-15   & 2  & 002100028910289891398946289406343554  \\
-16   & 1  & 002100028910289891398946289424343540  \\
-17   & 0  & 002100028910289891398984289840343400  \\
-17   & 2  & 002121028984289891398946289406343554  \\
-18   & 1  & 002100028910289891398984289891343434  \\
-19   & 0  & 002121028984289891398984289840343400  \\
-20   & 1  & 002121028984289891398984289891343434  \\
-21   & 0  & 212121398984289891398984289891343434  \\
\hline
\end{tabular}%3_1#3_1
}

\resizebox{\linewidth}{!}{
\begin{tabular}{|c|c|r|}
\hline
\multicolumn{3}{|c|}{$m(3_1)\#m(3_1)$}                  \\
\hline
tb    & rot  & Minimal Mosaic                        \\
\hline
3     & 0  & 002100029710297971379794037940003400  \\
2     & 1  & 002100029710297971379794037991003434  \\
1     & 0  & 002100029710297971379794243991355434  \\
1     & 2  & 002100029710297971639794627991343434  \\
0     & 1  & 002100029710297971379794287991343434  \\
0     & 3  & 002551029124297971639794627991343434  \\
-1    & 0  & 002121029746297916379794287991343434  \\
-1    & 2  & 002121029784297971639794627991343434  \\
-2    & 1  & 002121029784297971379794287991343434  \\
-3    & 0  & 212121399784297971379794287991343434  \\
\hline
\end{tabular}%m(3_1)#m(3_1)
}

\resizebox{\linewidth}{!}{
\begin{tabular}{|c|c|r|}
\hline
\multicolumn{3}{|c|}{$4_1$}                            \\
\hline
tb    & rot  & Minimal Mosaic                        \\
\hline
-3    & 0  & 000000021210297971379466037594003540  \\
-4    & 1  & 000000002100028910299971379794034340  \\
-5    & 0  & 000000002100028710298971379794034340  \\
-5    & 2  & 000000002100028910289791394346035554  \\
-6    & 1  & 000000002100028710289791398946034354  \\
-6    & 3  & 000000002100029710289991398984034340  \\
-7    & 0  & 000000002100028910289791398784034340  \\
-7    & 2  & 000000002100028710289791398984034340  \\
-7    & 4  & 000000002551029124289991398984034340  \\
-8    & 1  & 000000002121028784289791398946034354  \\
-8    & 3  & 000000002121029784289991398984034340  \\
-8    & 5  & 000210212891399984063991062984034340  \\
-9    & 0  & 000000002121028984289791398784034340  \\
-9    & 2  & 000000002121028784289791398984034340  \\
-9    & 4  & 000021021284289891399984243940355400  \\
-10   & 1  & 000000021210287891397984289891343434  \\
-10   & 3  & 000021021284289891399984243991355434  \\
-10   & 5  & 000210212891399984277991398984034340  \\
-11   & 0  & 000021021284287891397984289840343400  \\
-11   & 2  & 000021021284289891377984289840343400  \\
-11   & 4  & 000210212891399984287991388984034340  \\
-11   & 6  & 021210289791399984289991398984034340  \\
-12   & 1  & 000021021284287891397984289891343434  \\
-12   & 3  & 002121027984289891377984289840343400  \\
-12   & 5  & 021210288891399984277991398984034340  \\
-13   & 0  & 002121027984287891397984289891343434  \\
-13   & 2  & 002121027984289891377984289891343434  \\
-13   & 4  & 021210288891399984287991388984034340  \\
-14   & 1  & 002121028784288791398984289891343434  \\
-15   & 0  & 212121398784288791398984289891343434  \\
\hline
\end{tabular}%4_1
}

\resizebox{\linewidth}{!}{
\begin{tabular}{|c|c|r|}
\hline
\multicolumn{3}{|c|}{$5_1$}                            \\
\hline
tb    & rot  & Minimal Mosaic                        \\
\hline
-10   & 1  & 000000002100029710298991379946034354  \\
-11   & 0  & 000000002551029124298991379946034354  \\
-11   & 2  & 000000002100029710298991379984034340  \\
-12   & 1  & 000000002121029784298991379946034354  \\
-12   & 3  & 000210002460029160298991379984034340  \\
-13   & 0  & 000000021210289971399894243991355434  \\
-13   & 2  & 000000002121029784298991379984034340  \\
-14   & 1  & 000000021210289971399894287991343434  \\
-14   & 3  & 000210002871028894298991379946034354  \\
-15   & 0  & 000021021246289916399894287991343434  \\
-15   & 2  & 000021021284289971399894287940343400  \\
-15   & 4  & 000210002871028894298991379984034340  \\
-16   & 1  & 000021021284289971399894287991343434  \\
-16   & 3  & 000210212871398894298991379984034340  \\
-17   & 0  & 002121028846289916399894287991343434  \\
-17   & 2  & 002121027984289971399894287991343434  \\
-17   & 4  & 021210287871388894298991379984034340  \\
-18   & 1  & 002121028884289971399894287991343434  \\
-18   & 3  & 021210288871398894298991379984034340  \\
-19   & 0  & 212121398884289971399894287991343434  \\
\hline
\end{tabular}%5_1
}

\resizebox{\linewidth}{!}{
\begin{tabular}{|c|c|r|}
\hline
\multicolumn{3}{|c|}{$m(5_1)$}                         \\
\hline
tb    & rot  & Minimal Mosaic                        \\
\hline
3     & 0  & 000000025100062910299791379946034354  \\
2     & 1  & 000000002100028910299791379946034354  \\
1     & 0  & 000000002100028910299791379984034340  \\
1     & 2  & 000021251246629916397994039840003400  \\
0     & 1  & 000000002121028984299791379946034354  \\
0     & 3  & 000210255971625994662791398984034340  \\
-1    & 0  & 000000002121028984299791379984034340  \\
-1    & 2  & 000021251246629916397994289840343400  \\
-1    & 4  & 021210289791397994284391395546035554  \\
-2    & 1  & 000000021210289971397994289891343434  \\
-2    & 3  & 002121028984299791639946628406343554  \\
-3    & 0  & 000021021246289916397994289891343434  \\
-3    & 2  & 000210212791398984299791379984034340  \\
-3    & 4  & 021210289891397466289166397946034354  \\
-4    & 1  & 000021021284289971397994289891343434  \\
-4    & 3  & 021210279791398984299791379984034340  \\
-5    & 0  & 002121028846289916397994289891343434  \\
-5    & 2  & 002121027984289971397994289891343434  \\
-6    & 1  & 002121028884289971397994289891343434  \\
-7    & 0  & 021210287881397984288791398984034340  \\
\hline
\end{tabular}%m(5_1)
}

\resizebox{\linewidth}{!}{
\begin{tabular}{|c|c|r|}
\hline
\multicolumn{3}{|c|}{$5_2$}                            \\
\hline
tb    & rot  & Minimal Mosaic                        \\
\hline
-8    & 1  & 000210025971062994299971379794034340  \\
-9    & 0  & 000000251210629891397946039406003554  \\
-9    & 2  & 002100028910299971379794037940003400  \\
-10   & 1  & 000000002100258910629791398946034354  \\
-10   & 3  & 002100028910299971639794627940343400  \\
-11   & 0  & 000000002100258910629791398984034340  \\
-11   & 2  & 000000002100028910289791398946034354  \\
-12   & 1  & 000000002100028910289791398984034340  \\
-12   & 3  & 000210002891028984299771379984034340  \\
-13   & 0  & 000000002121258984629791398984034340  \\
-13   & 2  & 000000002121028984289791398946034354  \\
-13   & 4  & 021210287891379984299771379984034340  \\
-14   & 1  & 000000002121028984289791398984034340  \\
-14   & 3  & 000210002791028984289791398946034354  \\
-15   & 0  & 000000021210289891397984289891343434  \\
-15   & 2  & 000021251284629891397984289840343400  \\
-15   & 4  & 021210287791379984289791398946034354  \\
-16   & 1  & 000021021284289891397984289840343400  \\
-16   & 3  & 002121028984289791398846289406343554  \\
-17   & 0  & 000021021284289891397984289891343434  \\
-17   & 2  & 002100028910289791398884289891343434  \\
-18   & 1  & 002121027984289891397984289891343434  \\
-19   & 0  & 002121028884289891397984289891343434  \\
-19   & 2  & 002121028984289791398884289891343434  \\
-20   & 1  & 212121398884289891397984289891343434  \\
\hline
\end{tabular}%5_2
}

\resizebox{\linewidth}{!}{
\begin{tabular}{|c|c|r|}
\hline
\multicolumn{3}{|c|}{$m(5_2)$}                         \\
\hline
tb    & rot  & Minimal Mosaic                        \\
\hline
1     & 0  & 000000002100029710298971379794034340  \\
0     & 1  & 000000002121029746298916379794034340  \\
-1    & 0  & 000000002121029784298971379794034340  \\
-1    & 2  & 000000021210297971639894627991343434  \\
-2    & 1  & 000000021210297971379894287991343434  \\
-2    & 3  & 000210212891399946298916379846034354  \\
-3    & 0  & 000021021246297916379894287991343434  \\
-3    & 2  & 000021021284297971639894627991343434  \\
-4    & 1  & 000021021284297971379894287991343434  \\
-4    & 3  & 002121027984297971639894627991343434  \\
-5    & 0  & 000210212891399984288991379984034340  \\
-5    & 2  & 000210212871399894289991398984034340  \\
-6    & 1  & 002121028884297971379894287991343434  \\
-6    & 3  & 021210279891398984298991379984034340  \\
-7    & 0  & 002121028984297791379984289891343434  \\
-7    & 2  & 002121028984289791399784287991343434  \\
-8    & 1  & 212121398984289791399784287991343434  \\
\hline
\end{tabular}%m(5_2)
}

\resizebox{\linewidth}{!}{
\begin{tabular}{|c|c|r|}
\hline
\multicolumn{3}{|c|}{$6_1$}                            \\
\hline
tb    & rot  & Minimal Mosaic                        \\
\hline
-5    & 0  & 021000297100379910299791379946034354  \\
-6    & 1  & 000210255971602994629791398946034354  \\
-7    & 0  & 000210002971258994629791398946034354  \\
-7    & 2  & 021000289121397946299916379794034340  \\
-8    & 1  & 000210002891028984299791379946034354  \\
-9    & 0  & 000210212891398984299791379946034354  \\
-9    & 2  & 000210002891028984299791379984034340  \\
-10   & 1  & 000210212891398984299791379984034340  \\
-10   & 3  & 021210287891379984299791379984034340  \\
-11   & 0  & 021000287121397984289791398984034340  \\
-11   & 2  & 021000289121377984289791398984034340  \\
-12   & 1  & 021210287791397984289791398984034340  \\
-13   & 0  & 021210287881397984289791398984034340  \\
-13   & 2  & 021210287891397984288791398984034340  \\
\hline
\end{tabular}%6_1
}

\resizebox{\linewidth}{!}{
\begin{tabular}{|c|c|r|}
\hline
\multicolumn{3}{|c|}{$m(6_1)$}                         \\
\hline
tb    & rot  & Minimal Mosaic                        \\
\hline
-3    & 0  & 000210025971295894662971379794034340  \\
-4    & 1  & 000210002971029846298916379794034340  \\
-5    & 0  & 000210002871029894298971379794034340  \\
-5    & 2  & 000210002891029984298991379946034354  \\
-6    & 1  & 000210212871399894298971379794034340  \\
-6    & 3  & 000210002891029984298991379984034340  \\
-7    & 0  & 021210279871399894298971379794034340  \\
-7    & 2  & 000210212971399894289991398984034340  \\
-7    & 4  & 000210212891399984298991379984034340  \\
-8    & 1  & 021210288871399894298971379794034340  \\
-8    & 3  & 021210279891399984298991379984034340  \\
-9    & 2  & 021210288971399894289991398984034340  \\
-9    & 4  & 021210288891399984298991379984034340  \\
\hline
\end{tabular}%m(6_1)
}

\resizebox{\linewidth}{!}{
\begin{tabular}{|c|c|r|}
\hline
\multicolumn{3}{|c|}{$7_1$}                            \\
\hline
tb    & rot  & Minimal Mosaic                        \\
\hline
-14   & 1  & 000210002971029894298991379946034354  \\
-15   & 0  & 000210212971399894298991379946034354  \\
-15   & 2  & 000210002971029894298991379984034340  \\
-16   & 1  & 000210212971399894298991379984034340  \\
-17   & 0  & 021210279971399894298991379984034340  \\
-17   & 2  & 021210287971389894298991379984034340  \\
-18   & 1  & 021210288971399894298991379984034340  \\
\hline
\end{tabular}%7_1
}

\resizebox{\linewidth}{!}{
\begin{tabular}{|c|c|r|}
\hline
\multicolumn{3}{|c|}{$m(7_1)$}                         \\
\hline
tb    & rot  & Minimal Mosaic                        \\
\hline
5     & 0  & 021210299971397994299791379946034354  \\
4     & 1  & 021000289100397910299791379946034354  \\
3     & 0  & 021000289100397910299791379984034340  \\
3     & 2  & 021210289791397994299791379946034354  \\
2     & 1  & 021000289121397984299791379946034354  \\
1     & 0  & 021000289121397984299791379984034340  \\
1     & 2  & 021210289891397974299791379946034354  \\
0     & 1  & 021210289791397984299791379984034340  \\
-1    & 0  & 021210289881397984299791379984034340  \\
\hline
\end{tabular}%m(7_1)
}

\resizebox{\linewidth}{!}{
\begin{tabular}{|c|c|r|}
\hline
\multicolumn{3}{|c|}{$7_2$}                            \\
\hline
tb    & rot  & Minimal Mosaic                        \\
\hline
-10   & 1  & 021210297971379994299791379946034354  \\
-11   & 0  & 251210629891397946299716379946034354  \\
-11   & 2  & 021210289971397994299971379794034340  \\
-12   & 1  & 021210289891397946299716379946034354  \\
-13   & 0  & 021000289100397910289791398946034354  \\
-13   & 2  & 021210287891397984299791379946034354  \\
-14   & 1  & 021000289100397910289791398984034340  \\
-15   & 0  & 021000289121397984289791398946034354  \\
-15   & 2  & 021210289791397994289791398984034340  \\
-16   & 1  & 021000289121397984289791398984034340  \\
-17   & 0  & 021210289791397984289791398984034340  \\
-18   & 1  & 021210289881397984289791398984034340  \\
\hline
\end{tabular}%7_2
}

\resizebox{\linewidth}{!}{
\begin{tabular}{|c|c|r|}
\hline
\multicolumn{3}{|c|}{$m(7_2)$}                         \\
\hline
tb    & rot  & Minimal Mosaic                        \\
\hline
1     & 0  & 000210002971029894298971379794034340  \\
0     & 1  & 000210212971399894298971379794034340  \\
-1    & 0  & 021210279971399894298971379794034340  \\
-2    & 1  & 021210288971399894298971379794034340  \\
-3    & 0  & 021210289891399984298991379984034340  \\
\hline
\end{tabular}%m(7_2)
}

\resizebox{\linewidth}{!}{
\begin{tabular}{|c|c|r|}
\hline
\multicolumn{3}{|c|}{$8_1$}                            \\
\hline
tb    & rot  & Minimal Mosaic                        \\
\hline
-9    & 0  & 251210629891397984299791379946034354  \\
-10   & 1  & 021210289891397984299791379946034354  \\
-11   & 0  & 021210289891397984299791379984034340  \\
\hline
\end{tabular}%8_1
}

\resizebox{\linewidth}{!}{
\begin{tabular}{|c|c|r|}
\hline
\multicolumn{3}{|c|}{$m(8_1)$}                         \\
\hline
tb    & rot  & Minimal Mosaic                        \\
\hline
-3    & 0  & 021210297971379894298991379946034354  \\
-4    & 1  & 021210289971399894298971379794034340  \\
\hline
\end{tabular}%m(8_1)
}

\end{multicols}
}
\flushbottom
